# Supplementary material for: Query-Efficient Algorithm to Find all Nash Equilibria in a Two-Player Zero-Sum Matrix Game
Source: arXiv:2310.16236 source file (2024-09-04)
Supplement: Supplementary file 1 [file swordfish_appendix.tex]

\section{\sword/ Details and Experimental Results}\label{appendix:sword}
\subsection{Algorithm details}
\Cref{alg:swordfish} outlines \sword/ and its required subroutines.
Below, we use ``slice notation'' (as used in e.g. Python) to refer to partial vectors, e.g $\texttt{a[i:j]}$ refers to the vector comprised of the $i$ through $(j-1)$th components of $\texttt{a}$, and we assume vectors and arrays are $0$--indexed. We also denote the $(k,l)$th block submatrix (i.e. quadrant) of $B$ by $[B]_{kl}$. For instance, $[B]_{11}$ is the upper-left quadrant $[B]_{22}$ is the lower-right quadrant.
For convenience, we do not reference the tracking of sort indices or passing/returning of the mark and query matrices. 

\begin{algorithm2e}[ht!]\caption{{\sword/}}\label{alg:swordfish}
  \DontPrintSemicolon
  \SetDataSty{texttt}
  \SetKwInOut{Global}{Global}
  
  \SetKwData{DiagB}{diag\_b}
  \SetKwData{DiagM}{diag\_m}
  \SetKwData{False}{False}
  \SetKwData{True}{True}
  \SetKwData{Val}{val}
  \SetKwData{Queries}{queries}
  \SetKwData{Nullified}{nullified}
  \SetKwData{Move}{move}
  \SetKwData{None}{None}
  \SetKwData{NashOne}{nash\_1}
  \SetKwData{NashTwo}{nash\_2}

  \SetKwFunction{SwordfishBase}{swordfish}
  \SetKwFunction{Size}{size}
  \SetKwFunction{DiagSort}{diag\_sort}
  \SetKwFunction{Mark}{mark\_nullified}
  \SetKwFunction{NextMove}{next\_move}
  \SetKwFunction{Compare}{compare}
  
  \SetKwProg{Fn}{Function}{:}{}
  \Global{\Nullified}
  \Fn{\SwordfishBase{$B$}}{
        $n$ $\gets$ \Size{$B$}\;
        \DiagB, $B$ $\gets$ \DiagSort{$B$}\nllabel{ln:bruteforce}\;
        $(r,\: c) \gets (n-1,\: 0)$\;
        \While(  \tcp*[h]{until we exit the quadrant}\nllabel{ln:quickmove}){$r \geq \frac{n}{2}$ \textbf{and} $c<\frac{n}{2}$}{
            \Val $\gets B_{rc}$ \;
            \DiagM $\gets$   \texttt{diag\_b[c:r]}  \tcp{diagonal for submatrix of interest}
            \Mark{\Val, \DiagM}\;  
            $(r,\: c)  \gets (r,\: c) +$ \NextMove{$r,\:c$}
        }
        \If(  \tcp*[h]{up exit}){$c<\frac{n}{2}$}{
            $C_2 \gets$ $[B]_{11}$\;
        }
        \ElseIf(  \tcp*[h]{right exit}){$r \geq \frac{n}{2}$}{
            $C_2 \gets$ $[B]_{22}$\;
        }
        \Else(  \tcp*[h]{up-right exit}){
            $C_2 \gets$ \None\;
        }
        \NashOne $\gets$ \SwordfishBase{$[B]_{21}$}\;
        \NashTwo $\gets$ \SwordfishBase{$C_2$}\;
        \KwRet \Compare{\NashOne, \NashTwo}  \tcp{Retain one PSNE using \Cref{cor:2x2elim}}
  }
  \;
  \Fn{\Mark{\Val, \DiagM}}{
    $m \gets$ \Size{\DiagM}\;
    \For{$k=0$ \KwTo $m$ \nllabel{ln:bestmove}}{
        \If{\upshape\texttt{diag\_m[k]} $\leq$ \Val}{
            \texttt{nullified[k, 0]} $\gets$ \True\tcp{mark entries in first column}
        }
        \If{\upshape\texttt{diag\_m[k]} $\geq$ \Val}{
            \texttt{nullified[m-1, k]} $\gets$ \True\tcp{mark entries in last row}
        }
    }
  }
  \;
  \Fn{\NextMove{$r,\:c$}}{
    \Move $\gets (0,\: 0)$\;
    \If{\textbf{all}{\upshape(\texttt{nullified[:n/2,c]})}}{
     \Move $\gets$ \Move + $(0,\: 1)$  \tcp{can move right}
    }
    \If{\textbf{all}{\upshape(\texttt{nullified[r,n/2+1:]})}}{
     \Move $\gets$ \Move + $(-1,\:0)$  \tcp{can move up}
    }
    \KwRet \Move\;
  }
\end{algorithm2e}

\begin{figure}[ht]
\centering
\includegraphics[width=0.9\textwidth]{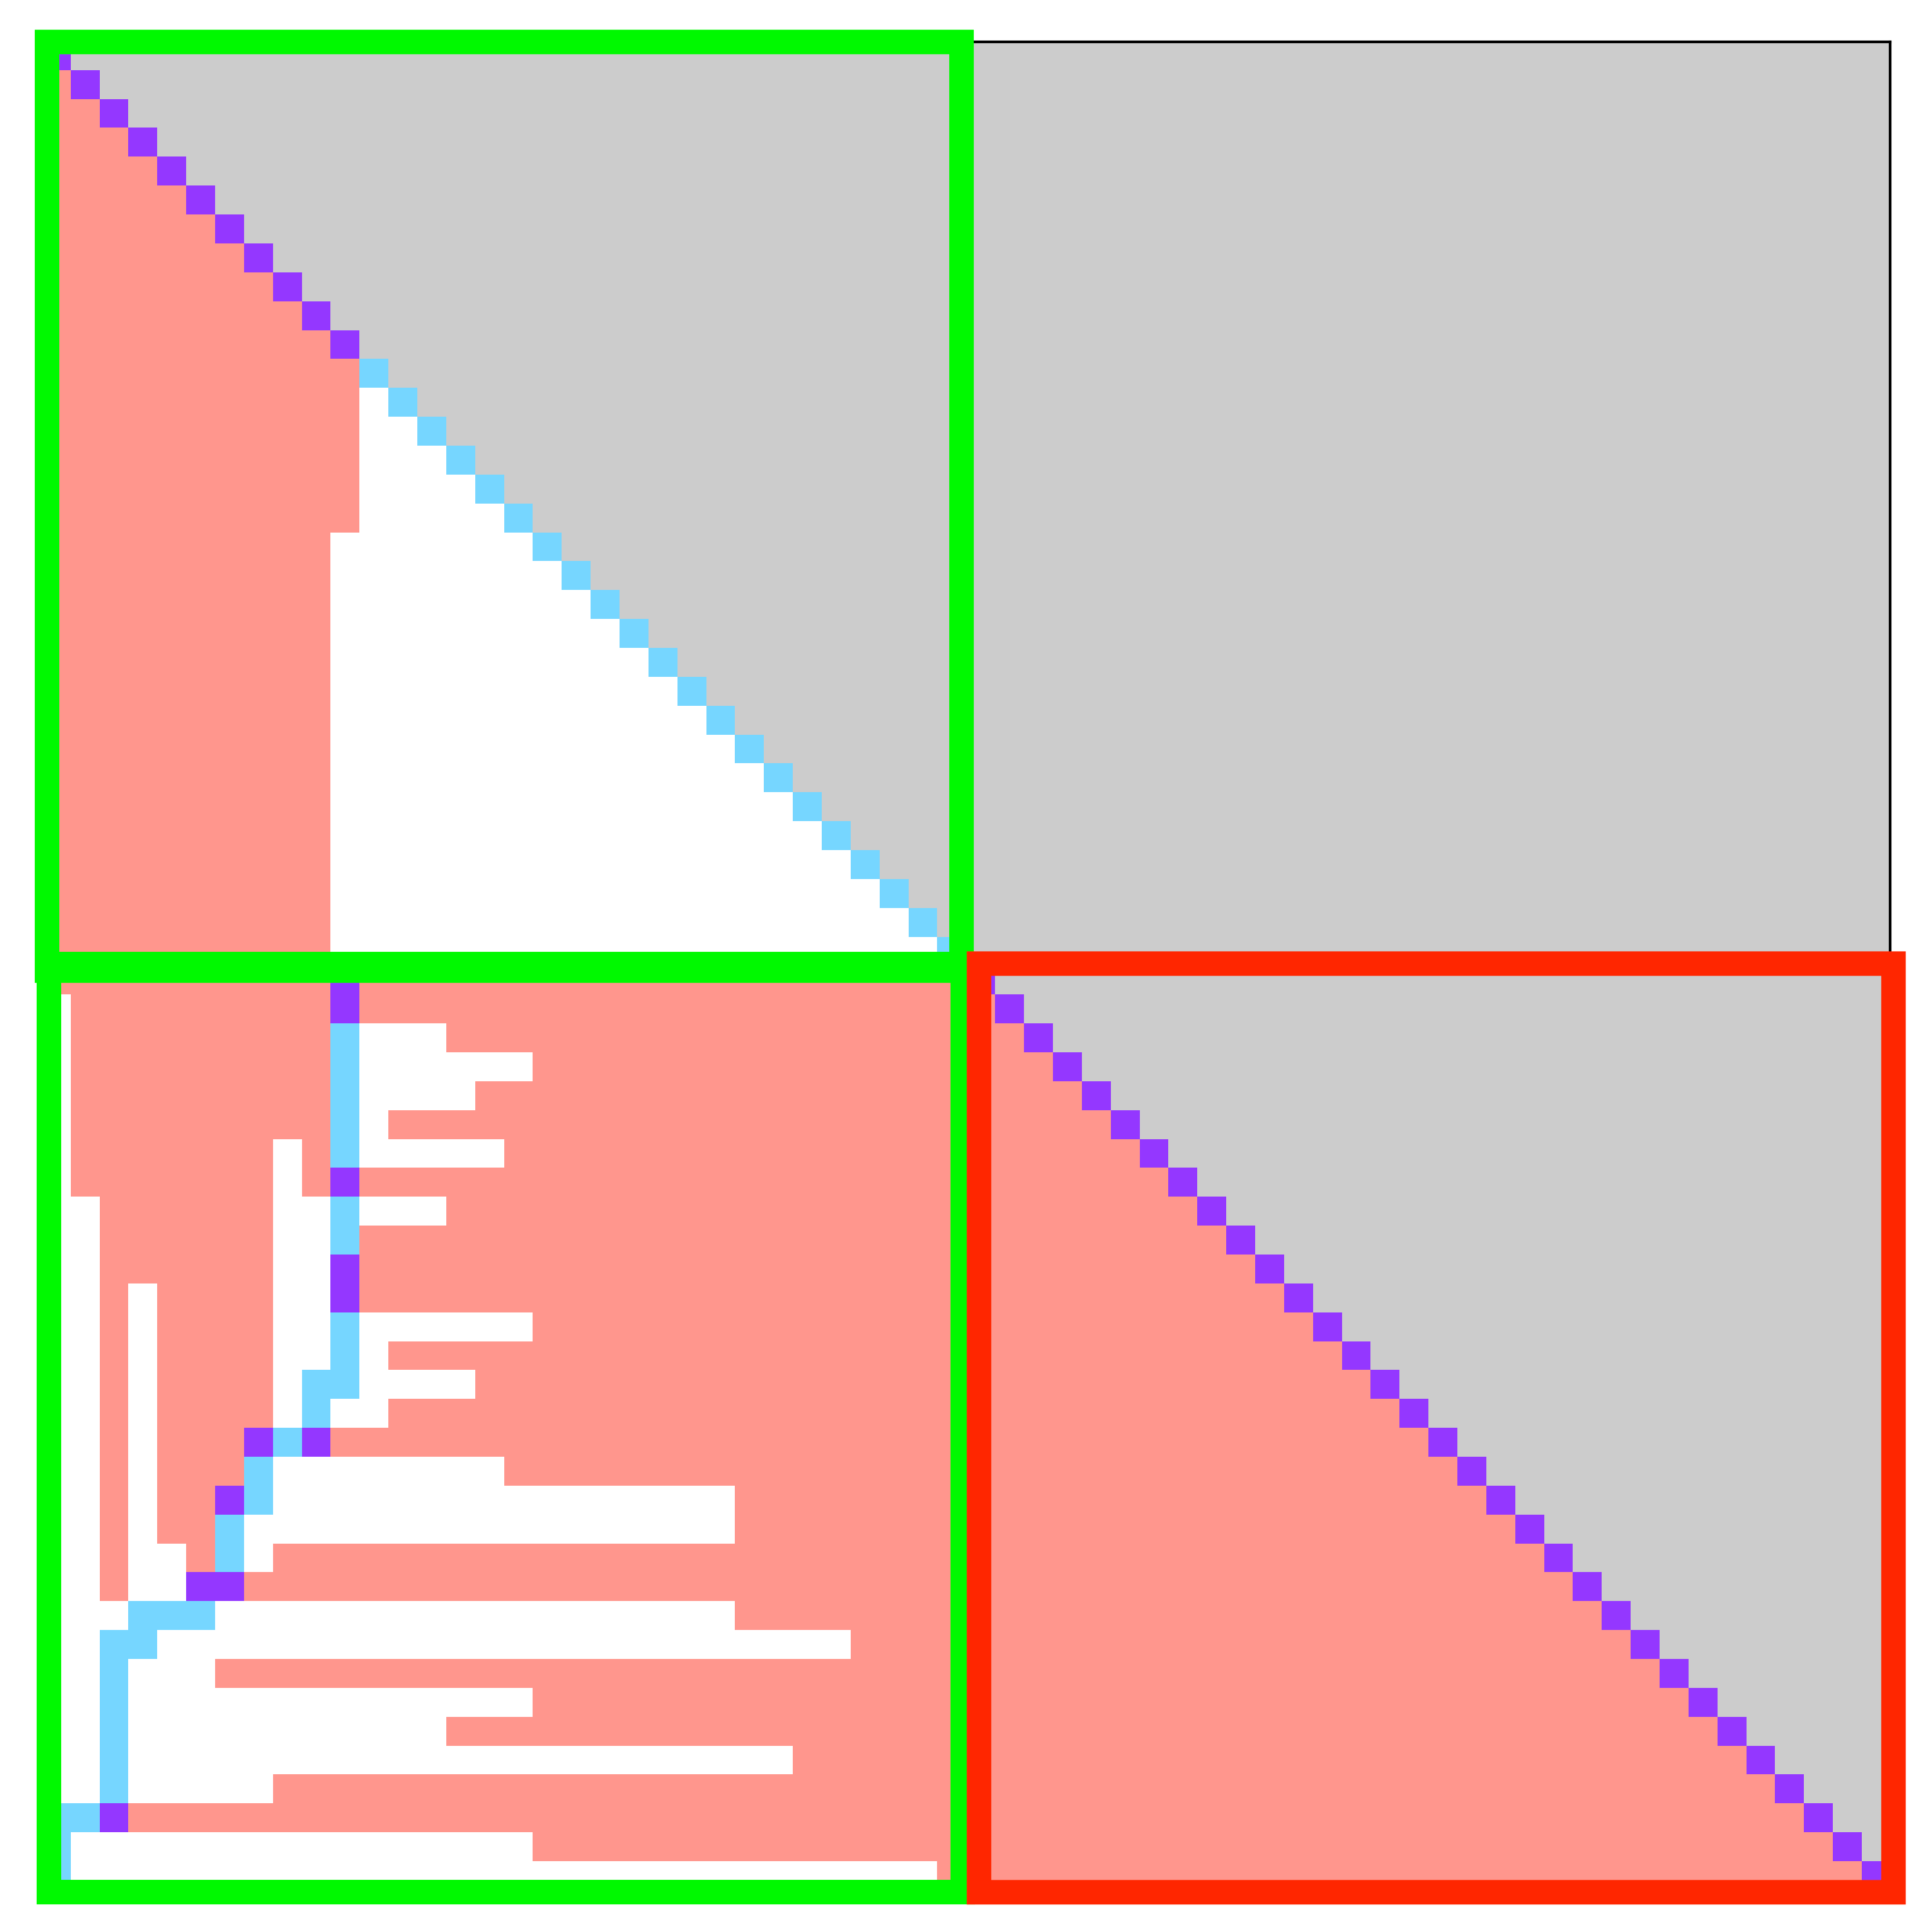}
\caption{An example end result of one stage of \sword/ with $n=2^6$. The red and gray cells represent entries of $B$ that have been nullified, while the blue cells represent entries  that have been queried (purple cells have both been marked inactive and been queried). After exiting to the upper-left quadrant, the lower-right quadrant is completely nullified, leaving the two subproblems (in green squares) to be solved.}
\label{fig:swordfish_big}
\end{figure}

\subsection{Refined complexity analysis}
As before, let us define $s(n)$ to be the number of queries required by \sword/ for an $n\times n$ matrix, and let $\shat(n)$ be the number of queries required by \sword/ if we pass in a matrix with a ``pre-queried'' diagonal, i.e. the case where the matrix is already diagonally queried and sorted. This leads to the system of recurrences
\[
s(n)\leq 2n + s(n/2)+\shat(n/2),\quad\shat(n)\leq n + s(n/2)+\shat(n/2)\:.
\]
For $n=2$, an extra comparison query is not needed. Thus, solving this system of recurrences with $s(2)=3$ and $\shat(2)=1$ gives
\begin{equation}\label{eq:sword_compl_bound}
s(n)\leq \frac{3}{2} n\log{n},\quad \shat(n) \leq \frac{3}{2} n \log{n} - n\:.
\end{equation}
\subsection{Experimental results}
Given the sample complexity bound in \Cref{eq:sword_compl_bound}, there are many optimizations that can be made to \sword/ that considerably reduce the number of queries required in practice.
Below, we list some of these optimizations (roughly) in order of effectiveness; though this is certainly not an exhaustive list.
Each optimization is a flag that can be toggled in the Python \sword/ implementation available at \url{https://github.com/QueryEfficientSODA2024/swordfish}.
\begin{itemize}
    \item \texttt{brute\_force}: Before executing \cref{ln:bruteforce}, if the number of remaining non-nullified entries in $B$ is less than some number $b(n)$, query each non-nullified entry and return the PSNE, if it exists.
    Here, $b(n)$ can be a constant, a function of the current submatrix size, or a function of the original matrix size.
    We conjecture that correctly choosing $b(n)$ may be necessary to reduce the theoretical query complexity below $\bigO(n\log n).$
    \item \texttt{quick\_mark}: Before entering the loop in \cref{ln:quickmove}, mark all possible entries of $B$ that can be nullified by previous queries as nullified. 
    This optimization reduces queries in the lower-left quadrant subproblems, as the previous query path gets ``scrambled'' once that quadrant gets diagonally sorted, and entries on the path are thereby able to nullify new entries.
    \item \texttt{recycle}: for a lower-left quadrant subproblem, before diagonally sorting in \cref{ln:bruteforce}, construct a partial diagonal from the parent problem's already-queried entries; this allows for fewer than $n$ new queries to construct a diagonal to be sorted.
    Computing this partial diagonal requires computing the \textit{maximum bipartite matching} of the graph induced by the queried entries of $B$.
    We do so using the Hopcroft–Karp algorithm \citep{hopcroft52Algorithm1973}, available in the \texttt{scipy.sparse} submodule.
    \item \texttt{quick\_move}: in \cref{ln:quickmove}, immediately move without querying another entry, if possible; i.e., if there are $n/2$ nullified entries (via earlier queries) at the beginning of the column or end of the row. 
\end{itemize}
In order to fairly compare these optimizations, we use the following two metrics to measure queries of the input matrix.
\begin{itemize}
    \item \textbf{unique queries}: how many unique entries of $A$ were queried by \sword/.
    \item \textbf{attempted queries}: how many times \sword/ queried an entry (or would have queried an entry) from $A$.
    In other words, these are queries that would have been made, given that the previous history of queries was unavailable (but not necessarily the knowledge of nullified entries).
    For example, the \texttt{recycle} optimization reduces unique queries, but is not (generally) guaranteed to reduce attempted queries, as it requires knowledge of the previous query path.
    The attempted queries metric is useful as it is more indicative of which optimizations may be mathematically proven to be effective, as reasoning about specific queries during the algorithm is challenging.
\end{itemize}

To illustrate the effectiveness of these optimizations in practice, we ran \sword/ against the following 4 problem classes:
\begin{itemize}
    \item \texttt{centered}: An entry is chosen uniformly at random as the Nash equilibrium, with value $V\sim\mathrm{Unif}([1/3, 2/3])$.
    The remaining row and column entries are then drawn i.i.d. from $\mathrm{Unif}([V,1])$ and $\mathrm{Unif}([0,V])$, respectively.
    \item \texttt{skewed}: As above, except we now draw $V\sim\mathrm{Unif}([0, 1/3] \cup [2/3, 1])$.
    \item \texttt{binary}: An entry is chosen uniformly at random as the Nash equilibrium, and assigned value $1/2$.
    Its row and column entries are filled with $1$s and $0$s, respectively, and the rest of the matrix is drawn i.i.d. from $\{0,1\}$.
    \item \texttt{curved} Each entry $(i, j)$ is initially set proportional to $5i + j$ and then perturbed with i.i.d. noise.
    A Nash row $\istar$ is selected from the last $n/2$ rows, and the column $(\jstar)$ corresponding to its minimum is then scaled to make $(\istar, \jstar)$ a PSNE.
\end{itemize}

Below, \Cref{fig:sword_opts} shows the effectiveness of each optimization on the \texttt{random\_centered} problem type, where we normalize the query complexity to the recurrence bound \eqref{eq:sword_compl_bound}.
Using the \texttt{brute\_force} optimization alone reduces the unique queries to below 50\% of the bound \eqref{eq:sword_compl_bound} for $n=2^{10}$.
\begin{figure}[ht!]
\centering
\includesvg[width=0.98\textwidth]{graphics/swordfish_all_opts_comparison.svg}
\caption{``Boxen plot'' of the effectiveness of different \sword/ optimizations for \texttt{random\_centered} matrices. For each $n$, each algorithm was run on the same $200$ input matrices. The \texttt{brute\_force} optimization uses $b(n)=2\log n$.}
\label{fig:sword_opts}
\end{figure}

In \Cref{fig:sword_grid} we demonstrate the effect of enabling all 4 optimizations, run against all 4 problem types.
\begin{figure}[ht!]
\centering
\includesvg[width=\textwidth]{graphics/swordfish_all_types_comparison.svg}
\caption{``Boxen plot'' of the effectiveness of combined \sword/ optimizations across different problem types. For each problem type and for each $n$, each algorithm was run on the same $500$ input matrices.}
\label{fig:sword_grid}
\end{figure}
In contrast to \Cref{fig:sword_opts}, enabling all optimizations further reduces unique queries on the \texttt{random\_centered} problem type to under 35\% of the bound \eqref{eq:sword_compl_bound} for $n=2^{10}$.
These figures suggest that it may be able to reduce the proven query complexity of \sword/ or related algorithms to $O(n)$ or $O(n \log(\log n))$, through better algorithm design and/or a more refined analysis.
