# Supplementary material for: Query-Efficient Algorithm to Find all Nash Equilibria in a Two-Player Zero-Sum Matrix Game
Source: arXiv:2310.16236 source file (2024-09-04)
Supplement: Supplementary file 2 [file appendix.tex]

\section{Omitted proofs}
