# Supplementary material for: Query-Efficient Algorithm to Find all Nash Equilibria in a Two-Player Zero-Sum Matrix Game
Source: arXiv:2310.16236 source file (2024-09-04)
Supplement: Supplementary file 3 [file old_appendix.tex]

 \section{Omitted Proofs of Section \ref{sec:technical}}
\subsection{Proof of Lemma \ref{Unique-NE-submatrix}}\label{appendix:lemma2}
%\arnab{Need to finish the section.}
In the following argument, let $\simplex_\calI$ be the probability simplex over a set of indices $\calI$. 

Let $(\xstar,\ystar)$ be the unique Nash equilibrium 
of $A\in\bbR^{n\times n}$. Suppose that $M$ is a sub-matrix of $A$ with row indices $\calX$ and column indices $\calY$, and that $\supp(\xstar)\subseteq \calX$ and $\supp(\ystar)\subseteq \calY$. 
 Let $(\widehat x,\widehat y)\in \simplex_{\calX}\times \simplex_{\calY}$ such that $(\widehat x)_i=(\xstar)_i$ for all $i\in \calX$ and $(\widehat y)_j=(\ystar)_j$ for all $j\in \calY$. 
 
 Due to \Cref{Nash-Shapley-lemma}, we have that \[\langle \xstar,A\ystar\rangle=\langle e_i, A\ystar\rangle\ \  \forall\  i\in\supp(\xstar)\quad\text{and}\quad\langle \xstar,A\ystar\rangle>\langle e_i, A\ystar\rangle\ \  \forall \ i\notin\supp(\xstar).\]
 Analogously, we have that \[\langle \xstar,A\ystar\rangle=\langle \xstar, Ae_j\rangle\ \ \forall \ j\in\supp(\ystar)\quad\text{and}\quad\langle \xstar,A\ystar\rangle<\langle \xstar, Ae_j\rangle\ \  \forall \ j\notin\supp(\ystar).\]
 Observe that $\supp(\widehat x)=\supp(\xstar)$ and $\supp(\widehat y)=\supp(\ystar)$ which implies that \[\langle \xstar,A\ystar\rangle=\langle \widehat x,M\widehat y\rangle,\quad  \langle e_i,A\ystar\rangle=\langle e_i,M\widehat y\rangle\ \  \forall \ i\in\calX\quad\text{and}\quad \langle \xstar,Ae_j\rangle=\langle \widehat x,Me_j\rangle\ \  \forall \ j\in\calY.\] 
 Now observe that \[\langle \widehat x,M\widehat y\rangle=\max_{i\in\calX}\langle e_i,M\widehat y\rangle \quad \text{and}
 \quad\langle \widehat x,M\widehat y\rangle=\min_{j\in\calY}\langle \widehat x,Me_j\rangle.\] Hence $(\widehat x,\widehat y)$ is a Nash equilibrium of $M$ which, in turn, implies that $V_A^\star=\langle \widehat x,M\widehat y\rangle=V_{M}^\star$. 
 
 Let us assume that $M$ has another Nash equilibrium $(x,y)$ such that, without loss of generality,  $x\neq \widehat x$.
 Now observe that $(x,\widehat y)$ is also a Nash equilibrium of $M$. 
 Therefore we deduce that $\langle x,Me_j\rangle=V_M^\star$ for all $j\in \supp(\widehat y)$. 
 
 Let $x^{(1)}\in\simplex_n$ such that $x^{(1)}_i=x_i$ for all $i\in\calX$.
 Now we have $\langle x^{(1)},Ae_j\rangle=V_A^\star$ for all $j\in \supp(\ystar)$.
 Let \[\Delta_1=\min_{j\notin \supp(\ystar)}\langle \xstar,Ae_j\rangle-V_A^\star\quad\text{and}\quad \Delta_2=\min_{j\notin \supp(\ystar)}\langle x^{(1)},Ae_j\rangle-V_A^\star.\]
 Since $\Delta_1>0$, there exists $\lambda\in(0,1)$ such that $(1-\lambda)\Delta_1+\lambda\Delta_2>0$. 
 
 Let $x^{(2)}=(1-\lambda)\cdot \xstar+\lambda\cdot x^{(1)}$. Now observe that for any $j\in \supp(\ystar)$, we have that \[\langle x^{(2)},Ae_j\rangle=(1-\lambda)\langle \xstar, Ae_j\rangle+\lambda\langle x^{(1)},Ae_j\rangle=(1-\lambda)\cdot V_A^\star+\lambda\cdot V_A^\star=V_A^\star.\] Similarly, observe that for any $j\notin \supp(\ystar)$, we have that \[\langle x^{(2)},Ae_j\rangle=(1-\lambda)\langle \xstar, Ae_j\rangle+\lambda\langle x^{(1)},Ae_j\rangle\geq (1-\lambda)\cdot (V_A^\star+\Delta_1)+\lambda\cdot (V_A^\star+\Delta_2)=V_A^\star+(1-\lambda)\Delta_1+\lambda\Delta_2>V_A^\star.\] Hence, we deduce that $x^{(2)}\in\arg\max_{x'\in \simplex_n}\min_{j\in[n]}\langle x',Ae_j\rangle$ which, in turn, implies that $(x^{(2)},\ystar)$ is also a Nash equilibrium of $A$. However, $x^{(2)}\neq \xstar$ which is a contradiction to the assumption that $A$ has a unique Nash equilibrium. Therefore $M$ has a unique Nash equilibrium---namely, $(\widehat x,\widehat y)$. 
\subsection{Proof of Lemma \ref{Unique-PSNE}}\label{appendix:lemma3}
Let $(x,y)$ be a Nash equilibrium of $M$.
Now observe that $(x,e_{\jstar})$ and $(e_{\istar},y)$ are also the Nash equilibrium of $M$.
This implies that $\supp(x)=\{\istar\}$ and $\supp(y)=\{\jstar\}$.
Hence $(e_{\istar},e_{\jstar})$ is the unique Nash equilibrium.


\section{Omitted Details of Theorem \ref{thm:lower-bound:new}} \label{appendix:lower}
%\arnab{Will make some minor changes here some time later.}
We complete the proof of the case $k>\frac{n}{2}$. Proving the following theorem suffices in this case.
\begin{theorem}\label{thm:lower-bound}
Let $\calA$ be any randomized algorithm that correctly computes the Nash equilibrium of the input matrix.
Let $\tau(M)$ denote the number of entries queried from the matrix $M$ by $\calA$.
Then, there exists an input matrix $A\in \bbR^{n\times n}$ with a unique Nash equilibrium $(\xstar,\ystar)$ such that $\bbE[\tau(A)]\geq \frac{n^2}{4}$ where $|\supp(\xstar)|=n$ and the randomness in $\tau(A)$ is due to $\calA$ only.
\end{theorem}
\begin{proof}
We prove \Cref{thm:lower-bound} using Yao's lemma. Let $E_{ij}$ denote the standard basis matrix with entry $(i,j)$ equal to $1$ and rest of the entries equal to $0$.
% Let $A^{i,j}$ denote an $n\times n$ matrix whose all entries have a value of $0$ except the entry $(i,j)$ and the entry $(i,j)$ has a value of $\frac{1}{2}$.
Denoting $\calM:=\{I+\frac{1}{2}E_{ij}\mid i,j\in[n]\}$, by Lemma~\ref{lem:no-two-matrix} (below), any input matrix in $\calM$ has a unique Nash equilibrium whose support size is $n$, and no two input matrices in $\calM$ have the same Nash equilibrium.
%; see \Cref{appendix:lower-omitted} for the proof of these facts.

% Fix a deterministic instance $A$ of the randomized algorithm $\calA$.
% As $A$ queries at most only $n^2/2-2 < n^2$ entries of the input matrix, by construction there exists a matrix $X'$ such that $A$ only queries entries in $X'$ with values in $\{0,1\}$. Denoting this set of indices as $S$, $A$ will then output the same pair $(x,y)$ for each of the input matrices in $\calM'=\{I+\frac{1}{2}E_{i,j}\mid(i,j)\notin S\}$, as each $X\in\calM'$ is equal to $X'$ on $S$.

% Since $(x,y)$ can be a Nash equilibrium of at most one instance in $\calM$, $A$ must be incorrect on at least $n^2 - (n^2/2 - 2) - 1 = n^2/2+1$ input matrices in $\calM$.
% Thus, if we draw $X\sim\text{Unif}(\calM)$, $A$ will return an incorrect pair with probability more than $1/2$.
% As this bound holds uniformly over algorithm instances of $\calA$, it holds for the best algorithm instance.
% Therefore, the probability of failure of the randomized algorithm $\calA$ is then more than $1/2$ for some input matrix $X$, as Yao's lemma states that
% \[
% \max_{X\in\calM}\bbP_\calA(\calA(X)\neq\text{Nash}(X)) \geq \min_{A\in\calA}\bbP_{X'\sim\text{Unif}(\calM)}(A(X')\neq\text{Nash}(X')) > \frac{1}{2}.
% \] 


Let us assume that the randomized algorithm $\calA$ is a distribution over a set $\calD$ of deterministic algorithms.
Fix a deterministic instance $\alg\in \calD$. We now claim that there is a subset $\calM_1\subseteq \calM$ of size $\frac{|\calM|}{2}$ such that $\alg$ queries at least $\frac{n^2}{2}$ entries from each input instance in $\calM_1$.
As $\alg$ computes the correct Nash equilibrium of the input matrix, by construction there exists a matrix $M\in \calM$ such that the first $\frac{n^2}{2}$ entries of $M$ queried by $\alg$ have values in $\{0,1\}$. Denoting this set of entries as $S$, $\alg$ will query all the entries in $S$ from each of the input matrices in $\calM_1=\{I+\frac{1}{2}E_{ij}\mid(i,j)\notin S\}$, as each $A\in\calM_1$ is equal to $M$ on $S$ and every matrix in $\calM_1$ has a different unique Nash equilibrium. Let $\tau(\alg,A)$ denote the number of queries taken by $\alg$ from an input matrix $A$. As $|\calM_1|=\frac{|\calM|}{2}$, we have $\mathbb{E}_{X\sim\text{Unif}(\calM)}[\tau(\alg,A)]\geq \frac{1}{2}\cdot \frac{n^2}{2}=\frac{n^2}{4}$. Hence, invoking Yao's lemma, we deduce that
\[
\max_{A\in\calM}\E[\tau(A)] \geq \min_{\alg\in\calD}\E_{A\sim\text{Unif}(\calM)}[\tau(\alg,A)] \geq \frac{n^2}{4},
\] 
which concludes the proof.
\end{proof}



%\subsection{Omitted details of \texorpdfstring{\Cref{thm:lower-bound}}{Theorem \ref{thm:lower-bound}}}\label{appendix:lower-omitted}
\begin{lemma}
    \label{lem:no-two-matrix}
    No two distinct matrices of the form $A=I+\frac{1}{2}E_{ij}$ for some $i,j\in [n]$ have the same (unique) Nash equilibrium $(\xstar,\ystar)$.
\end{lemma}
\begin{proof}
% message for ross: Sorry but I had to revert back to my proof as I found a small bug in your proof. It is fixable but in hindsight my proof is way more simple and elegant compared to yours. So let's stick to this proof.

Recall that $\mathcal{M}:=\{I+\frac{1}{2}E_{i,j}\mid i,j\in[n]\}$ be the set of all input instances where $I$ is the identity matrix. Now we show that no two input instances in $\mathcal{M}$ have the same unique Nash Equilibrium.

First let us consider $i_1,j_1\in[n]$ such that $i_1\neq j_1$. Now we construct a pair $(\xstar,\ystar)\in\simplex_n\times\simplex_n$. Let $(\xstar)_i=\frac{1}{n-1/2}$ for all $i\in [n]\setminus\{j_1\}$ and $(\xstar)_{j_1}=\frac{1/2}{n-1/2}$. Similarly let $(\ystar)_j=\frac{1}{n-1/2}$ for all $j\in [n]\setminus\{i_1\}$ and $(\ystar)_{i_1}=\frac{1/2}{n-1/2}$. Now we claim that $(\xstar,\ystar)$ is the unique Nash Equilibrium of $A=I+\frac{1}{2}E_{i_1,j_1}$. First observe that $\langle \xstar,Ae_j\rangle=\frac{1}{n-1/2}$ for all $j\in[n]$ and $\langle e_i,A\ystar\rangle=\frac{1}{n-1/2}$ for all $i\in[n]$. Hence $(\xstar,\ystar)$ is a Nash Equilibrium of $A$ and $V^\star_{A}=\frac{1}{n-1/2}$. Now consider any pair $(x,y)\in\simplex_n\times \simplex_n$ which is also a Nash Equilibrium of $A$. Observe that $(x,\ystar)$ is also a Nash Equilibrium of $A$. This implies that $\langle x,Ae_j\rangle=V^\star_{A}$ for all $j\in [n]$. Hence we have $x_i=\frac{1}{n-1/2}$ for all $i\in [n]\setminus \{j_1\}$ and $x_{j_1}+\frac{x_{i_1}}{2}=\frac{1}{n-1/2}$ which implies that $x_{j_1}=\frac{1/2}{n-1/2}$. Therefore we have $x=\xstar$. Similarly observe that $(\xstar,y)$ is also a Nash Equilibrium of $A$. This implies that $\langle e_i,Ay\rangle=V^\star_{A}$ for all $i\in[n]$. Hence we have $y_j=\frac{1}{n-1/2}$ for all $j\in [n]\setminus \{i_1\}$ and $y_{i_1}+\frac{y_{j_1}}{2}=\frac{1}{n-1/2}$ which implies that $y_{i_1}=\frac{1/2}{n-1/2}$. Therefore we have $y=\ystar$.

Analogously, we can show that for any $i_1\in[n]$, $(\xstar,\ystar)$ is the unique Nash Equilibrium of $I+\frac{1}{2}E_{i_1,i_1}$ where $(\xstar)_i=\frac{1}{n-1/3}$ for all $i\in [n]\setminus\{i_1\}$, $(\xstar)_{i_1}=\frac{2/3}{n-1/3}$, $(\ystar)_j=\frac{1}{n-1/3}$ for all $j\in [n]\setminus\{i_1\}$ and $(\ystar)_{i_1}=\frac{2/3}{n-1/3}$. It is easy to observe that no two distinct matrices of the form $A=I+\frac{1}{2}E_{ij}$ for some $i,j\in [n]$ have the same (unique) Nash equilibrium $(\xstar,\ystar)$.


% Denote the supports of $\xstar,\ystar$ by $\calI$ and $\calJ$, respectively. Observe that
% \begin{align*}
% u:=& A^\top \xstar = \xstar + \frac{(\xstar)_i\cdot \mathbbm{1}\{i\in\calI\}}{2} e_j \\
% v:=& A \ystar = \ystar + \frac{(\ystar)_j\cdot \mathbbm{1}\{j\in\calJ\}}{2} e_i \:.
% \end{align*}
% Since $\xstar$ is a best response to $v$, it must be the case that
% \begin{subequations}
% \begin{empheq}[left={\calI\subseteq \supp(v)=\empheqlbrace}]{align}
% \calJ,&\quad\quad i\in\calJ\text{ or } j\notin \calJ  \label{eq:best_resp_I_case1}\\
% \calJ\cup\{i\},&\quad\quad i\notin \calJ,\: j\in \calJ  \label{eq:best_resp_I_case2}.
% \end{empheq}
% \end{subequations}
% Case \eqref{eq:best_resp_I_case2} implies $i\neq j$ so that
% \[
% v_i=\frac{1}{2}(\ystar)_j < (\ystar)_j = v_j.
% \]
% That is, action $i$ is suboptimal for $\xstar$ and thus is not included in $\calI$. Therefore, $\calI\subseteq\calJ$ holds in both cases.

% Analogously, since $\ystar$ is a best response to $u$, if $u$ does not have full support, $\calJ$ will not intersect $\supp(u)$. Thus, we have that
% \begin{subequations}
% \begin{empheq}[left={\supp(u)=[n]\text{ or }\empheqlbrace}]{align}
% \calI \cap \calJ =\emptyset,&\quad\quad j\in\calI\text{ or } i\notin \calI  \quad(\supp(u)=\calI)\label{eq:best_resp_J_case1}\\
% (\calI \cup \{j\}) \cap \calJ= \emptyset,&\quad\quad j\notin \calI,\: i\in \calI \quad(\supp(u)=\calI\cup\{j\})\label{eq:best_resp_J_case2}.
% \end{empheq}
% \end{subequations}
% Since $\calI\subseteq\calJ$, we have $\supp(u)=[n]$. In case \eqref{eq:best_resp_J_case1}, we have that $\calI=\calJ=[n]$.
% In case \eqref{eq:best_resp_J_case2} (again implying $i\neq j$), we have that $\calI=[n]\setminus \{j\}$ and $\calJ=[n]$; 
% However, this leads to a contradiction:
% the strategy $\ystar$ cannot be a full-support best response, since 
% \[
% u_j = \frac{1}{2}(\xstar)_i < (\xstar)_i = u_i,
% \]
% implying that $i$ is suboptimal for $\ystar$.

% Having shown $\xstar$ and $\ystar$ both have full support $[n]$, a short calculation via the principle of indifference ($A\ystar=A^\top \xstar=V_A^\star\cdot \mathbf{1}$) shows that the unique mixed-strategy Nash equilibrium is given by
% \begin{align*}
% \xstar &= \frac{1}{n-\alpha}\Par*{\ones - \alpha e_j},\quad \ystar = \frac{1}{n-\alpha}\Par*{\ones - \alpha e_i},
% \end{align*}
% where $\alpha=1/2$ for $i\neq j$ and $\alpha=1/3$ for $i=j$. It is easy to observe that every input matrix in $\mathcal{M}$ has a different unique Nash equilibrium.
\end{proof}

\section{Omitted Details of Section \ref{sec:upper}}\label{appendix:upper}
Here we provide an intuition for why an approach based on standard no-regret algorithms can end up with a gap dependence. Let us consider a simple multiplicative weight update based algorithm $\calA$ which does the following. In each round $t$, it maintains a weight vector $w_t\in \mathbb{R}^{n}$ where $w_1=\mathbf{1}$. In each round it sees a vector $x_t\in \mathbb{R}^{n}$ and updates $(w_{t+1})_i=(w_t)_i\cdot e^{\eta (x_t)_i}$ for all $i\in[n]$ where $\eta$ is some fixed parameter. Now let us consider this toy problem of finding $\arg\max\{a,b\}$. Let $a>b$. If we run the algorithm $\calA$ on a fixed vector $x=(a,b)$ in each round and declare $i$ as the $\arg\max\{a,b\}$ in round $t$ when $\frac{(w_t)_i}{(w_t)_1+(w_t)
_2}$ becomes greater than $1-\delta$ then $t$ needs to be proportional to $\frac{1}{a-b}$. Here $\delta$ is a confidence parameter which is close to zero.

Consider $\Delta\in (0,1)$. Now let us consider a matrix $A\in \mathbb{R}^{n\times n}$ such that $A_{1,1}=1$, $A_{1,j}=1+\Delta$ for all $j>1$, $A_{i,1}=1-\Delta$ for all $i>1$ and rest of the entries have a value $1$. Now due to the analysis of toy example, when both row and column player run the algorithm $\calA$, they can take $\Omega(\frac{n}{\Delta})$ distinct queries from the input matrix before they find the unique PSNE. If $\Delta<\frac{1}{n}$, then the query complexity can be as large as $\Omega(n^2)$.


% \arnab{Just adding my old proof below for the sake of completion.}
 % Recall that $\mathcal{M}:=\{I+A^{i,j}:i,j\in[n]\}$ be the set of all input instances where $I$ is the identity matrix. Now we show that no two input instances in $\mathcal{M}$ have the same Nash Equilibrium.

 % First let us consider $i_1,j_1\in[n]$ such that $i_1\neq j_1$. Now we construct a pair $(x^*,y^*)\in\simplex_n\times\simplex_n$. Let $x_i^*=\frac{1}{n-1/2}$ for all $i\in [n]\setminus\{j_1\}$ and $x_{j_1}^*=\frac{1/2}{n-1/2}$. Similarly let $y_j^*=\frac{1}{n-1/2}$ for all $j\in [n]\setminus\{i_1\}$ and $y_{i_1}^*=\frac{1/2}{n-1/2}$. Now we claim that $(x^*,y^*)$ is the unique Nash Equilibrium of $I+A^{i_1,j_1}$. First observe that $\langle x^*,Ae_j\rangle=\frac{1}{n-1/2}$ for all $j\in[n]$ and $\langle e_i,Ay^*\rangle=\frac{1}{n-1/2}$ for all $i\in[n]$. Hence $(x^*,y^*)$ is a Nash Equilibrium of $I+A^{i_1,j_1}$ and $V^*_{I+A^{i_1,j_1}}=\frac{1}{n-1/2}$. Now consider any pair $(x,y)\in\simplex_n\times \simplex_n$ which is also a Nash Equilibrium of $I+A^{i_1,j_1}$. Observe that $(x,y^*)$ is also a Nash Equilibrium of $I+A^{i_1,j_1}$. This implies that $\langle x,Ae_j\rangle=V^*_{I+A^{i_1,j_1}}$ for all $j\in [n]$. Hence we have $x_i=\frac{1}{n-1/2}$ for all $i\in [n]\setminus \{j_1\}$ and $x_{j_1}+\frac{x_{i_1}}{2}=\frac{1}{n-1/2}$ which implies that $x_{j_1}=\frac{1/2}{n-1/2}$. Therefore we have $x=x^*$. Similarly observe that $(x^*,y)$ is also a Nash Equilibrium of $I+A^{i_1,j_1}$. This implies that $\langle e_i,Ay\rangle=V^*_{I+A^{i_1,j_1}}$ for all $i\in[n]$. Hence we have $y_j=\frac{1}{n-1/2}$ for all $j\in [n]\setminus \{i_1\}$ and $y_{i_1}+\frac{y_{j_1}}{2}=\frac{1}{n-1/2}$ which implies that $y_{i_1}=\frac{1/2}{n-1/2}$. Therefore we have $y=y^*$.

% Next let us consider $i_1\in[n]$. Now we construct a pair $(x^*,y^*)\in\simplex_n\times\simplex_n$. Let $x_i^*=\frac{1}{n-1/3}$ for all $i\in [n]\setminus\{i_1\}$ and $x_{j_1}^*=\frac{2/3}{n-1/2}$. Similarly let $y_j^*=\frac{1}{n-1/3}$ for all $j\in [n]\setminus\{i_1\}$ and $y_{i_1}^*=\frac{2/3}{n-1/3}$. Now we claim that $(x^*,y^*)$ is the unique Nash Equilibrium of $I+A^{i_1,i_1}$. First observe that $\langle x^*,Ae_j\rangle=\frac{1}{n-1/3}$ for all $j\in[n]$ and $\langle e_i,Ay^*\rangle=\frac{1}{n-1/3}$ for all $i\in[n]$. Hence $(x^*,y^*)$ is a Nash Equilibrium of $I+A^{i_1,i_1}$ and $V^*_{I+A^{i_1,i_1}}=\frac{1}{n-1/3}$. Now consider any pair $(x,y)\in\simplex_n\times \simplex_n$ which is also a Nash Equilibrium of $I+A^{i_1,i_1}$. Observe that $(x,y^*)$ is also a Nash Equilibrium of $I+A^{i_1,i_1}$. This implies that $\langle x,Ae_j\rangle=V^*_{I+A^{i_1,i_1}}$ for all $j\in[n]$. Hence we have $x_i=\frac{1}{n-1/3}$ for all $i\in [n]\setminus \{i_1\}$ and $\frac{3x_{i_1}}{2}=\frac{1}{n-1/3}$ which implies that $x_{i_1}=\frac{2/3}{n-1/3}$. Therefore we have $x=x^*$. Similarly observe that $(x^*,y)$ is also a Nash Equilibrium of $I+A^{i_1,i_1}$. This implies that $\langle e_i,Ay\rangle=V^*_{I+A^{i_1,i_1}}$ for all $i\in[n]$. Hence we have $y_j=\frac{1}{n-1/3}$ for all $j\in [n]\setminus \{i_1\}$ and $\frac{3y_{i_1}}{2}=\frac{1}{n-1/3}$ which implies that $y_{i_1}=\frac{2/3}{n-1/3}$. Therefore we have $y=y^*$.

% \section{\sword/ Algorithm of Section~\ref{sec:deterministic}}\label{appendix:sword}
% First we describe the Phase-I of \sword/
% \begin{algorithm2e}[!ht]
% \caption{\sword/ Phase-I}
% \label{alg:sword1}
% \DontPrintSemicolon
% $n\gets$ number of rows of $A$,\: $B_1\gets A$,\: $\calS\gets \emptyset$\;
% Query all the diagonal entries of $A$\;
% \For{$k=1,2,\ldots,n-1$}{
%     % \If{$|\calX_t|=1$}{
%     % \KwRet $(\;\ihat,\:\jhat\;)$, where $\calX_t=\{\;\ihat\;\}$ and $\calY_t=\{\;\jhat\;\}$
%     % }
%     $\widehat i\gets \argmin_{i}(B_k)_{i,i}$ and $\widehat j\gets \argmax_{j}(B_k)_{j,j}$\;
%     Add the entries $(B_k)_{\widehat i,\widehat i}$ and $(B_k)_{\widehat j,\widehat j}$ to $\calS$\;
%     Query the entry $(B_{k})_{\widehat j, \widehat i}$\;
%     Create a sub-matrix $B_{k+1}$ of $B_k$ by first removing the row $\widehat i$ and the column $\widehat j$ from $B_k$.\;
%     Rearrange the rows and columns of $B_{k+1}$ so that the queried entries of $B_{k+1}$ become the diagonal entries of $B_{k+1}$.\;
% }
% Add the only entry in $B_n$ to $\calS$
% \end{algorithm2e}

% Next we describe the Phase-II of \sword/
% \begin{algorithm2e}[!ht]
% \caption{\sword/ Phase-II}
% \label{alg:sword2}
% \DontPrintSemicolon
% \textbf{Given:} Queried elements $\calS$ from Phase-I\;
% \textbf{Pre-processing each row:} If there are more than one queried elements in a row, retain the unique least queried element, if it exists, and remove rest of the queried elements from $\calS$\;
% \textbf{Pre-processing each column:} If there are more than one queried elements in a column, retain the unique highest queried element, if it exists, and discard rest of the queried elements from $\calS$\;
% $\widehat i\gets 2$, $\widehat j\gets 1$ and $s\gets |\calS|$\;
% Rearrange the rows and columns of $A$ so that the entries in $\calS$ become the diagonal entries $A_{1,1},A_{2,2},\ldots,A_{s,s}$ in an increasing order.\;
% \For{$k=1,2,\ldots$}{
%      \If{$|\calS|=1$}{
%      \KwRet the entry in $\calS$ as the PSNE of $A$
%      }
%      Query the entry $A_{\widehat i,\widehat j}$.\;
%      \If{$A_{\widehat i,\widehat j}<A_{\widehat j,\widehat j}$ and $A_{\widehat i,\widehat j}\leq A_{\widehat i,\widehat i}$}{
%       Remove the entry $A_{\widehat i,\widehat i}$ from $\calS$\;
%       $\widehat i\gets \widehat i+1$\;
%      }
%      \ElseIf{$A_{\widehat i,\widehat j}\geq A_{\widehat j,\widehat j}$ and $A_{\widehat i,\widehat j}> A_{\widehat i,\widehat i}$}{
%       Remove the entry $A_{\widehat j,\widehat j}$ from $\calS$\;
%       $\widehat j\gets \widehat i$\;
%       $\widehat i\gets \widehat i+1$\;
%      }
%      \ElseIf{$A_{\widehat i,\widehat j}\geq A_{\widehat j,\widehat j}$ and $A_{\widehat i,\widehat j}\leq A_{\widehat i,\widehat i}$}{
%       Remove the entries $A_{\widehat i,\widehat i}$ and $A_{\widehat j,\widehat j}$ from $\calS$\;
%       $\widehat j\gets \widehat i+1$\;
%       $\widehat i\gets \widehat i+2$\;
%      }
% }
% \end{algorithm2e}

\section{Modification of Algorithm \ref{alg:psne}}\label{appendix:modification-psne}
Using an identical analysis as that of Algorithm \ref{alg:psne}, one can show that Algorithm \ref{alg:psne-nm} finds the unique PSNE of a $n\times m$ matrix $A$ with probability at least $1-\delta$ by querying at most $O((n+m)\cdot\log(\frac{n+m}{\delta}))$ entries. 
\begin{algorithm2e}[!ht]
\caption{\psnealg/2($A$)}
\label{alg:psne-nm}
\DontPrintSemicolon
$n\gets$ number of rows of $A$,\: $\calX_1 \gets [n], \:\calY_1 \gets [m]$\;
\For{$t=1,2,\ldots$}{
    \If{$|\calX_t|=1$ and $|\calY_t|=1$}{
    \KwRet $(\;\ihat,\:\jhat\;)$, where $\calX_t=\{\;\ihat\;\}$ and $\calY_t=\{\;\jhat\;\}$
    }
    \If{$|\calX_t|=1$ }{
    \KwRet unique minimizer $(\;\ihat,\:\jhat\;)$ of row $\ihat$, where $\calX_t=\{\;\ihat\;\}$
    }
    \If{$|\calY_t|=1$}{
    \KwRet unique maximizer $(\;\ihat,\:\jhat\;)$ of column $\jhat$, where $\calY_t=\{\;\jhat\;\}$
    }
    $n_{t}\gets |\calX_t|$, $m_t\gets |\calY_t|$ and $\ell\gets 2\log(\frac{n^2+m^2}{\delta})$\;
    $\Xbar_t \gets\{x_1,x_2,\ldots, x_{\ell}\}$; $x_i$'s are drawn independently and uniformly at random from $\calX_t$ \label{recurse:line2}\;
    $\Ybar_t \gets \{y_1,y_2,\ldots, y_{\ell}\}$; $y_j$'s are drawn independently and uniformly at random from $\calY_t$ \label{recurse:line3}\;
    Query all the entries of $A$ in $\{(i,j):i\in\calX_t,j\in \Ybar_t\}\cup\{(i,j):i\in \Xbar_t,j\in \calY_t\}$\;
    
    %Query each $(i\:,j)$ in $\{\calX_t \times \Ybar_t\} \cup \{\Xbar_t\times  \calY_t\}$\;
    Choose the arguments $\ihat\in \argmax_{i\in\calX_t}\min_{j\in \Ybar_t}A_{i,j}$ and $\jhat\in \argmin_{j\in\calY_t}\max_{i\in \Xbar_t}A_{i,j}$\;
    Query all the entries of $A$ in $\{({i,\jhat}): i\in \calX_t\}\cup\{({\ihat,\:j}):j\in\calY_t\}$\;
    
    %Query each $(i,j)$ in $\{\calX_t \times \jhat\} \cup \{\ihat \times \calY_t\}$\;
    %\tcp{Sort Xt by j\_hat and Yt by i\_hat, take half}
    $\calX_{t+1}\gets \{i_1,i_2,\ldots, i_{\lfloor n_t/2\rfloor}\} \subseteq \calX_t=\{i_1,\ldots,i_{n_t}\}$,   where $A_{i_1,\jhat}\geq A_{i_2,\jhat}\geq \ldots \geq A_{i_{n_t},\jhat}$\;
    $\calY_{t+1}\gets \{j_1,j_2,\ldots, j_{\lfloor m_t/2\rfloor}\}\subseteq \calY_t=\{j_1,\ldots,j_{m_t}\}$, where $A_{\ihat,j_1}\leq A_{\ihat,j_2}\leq \ldots \leq A_{\ihat,j_{m_t}}$\;
}
\end{algorithm2e}
